# Supplementary material for: Quantum microwave parametric interferometer
Source: arXiv:2303.01026 ancillary file (2023-03-02)
Supplement: Supplementary file 1 [file QUMPI_Supplemental_Material.pdf]

# Supplemental Material: Quantum microwave parametric interferometer

F. Kronowetter,[1, 2, 3, *] F. Fesquet,[1, 2] M. Renger,[1, 2] K. Honasoge,[1, 2] Y. Nojiri,[1, 2]
K. Inomata,[4, 5] Y. Nakamura,[4, 6] A. Marx,[1] R. Gross,[1, 2, 7] and K. G. Fedorov[1, 2, †]

[1] *Walther-Meißner-Institut, Bayerische Akademie der Wissenschaften, 85748 Garching, Germany*
[2] *School of Natural Sciences, Technische Universität München, 85748 Garching, Germany*
[3] *Rohde & Schwarz GmbH & Co. KG, 81671 Munich, Germany*
[4] *RIKEN Center for Quantum Computing (RQC), Wako, Saitama 351-0198, Japan*
[5] *National Institute of Advanced Industrial Science and Technology, 1-1-1 Umezono, Tsukuba, Ibaraki, 305-8563, Japan*
[6] *Department of Applied Physics, Graduate School of Engineering, The University of Tokyo, Bunkyo-ku, Tokyo 113-8656, Japan*
[7] *Munich Center for Quantum Science and Technology (MCQST), 80799 Munich, Germany*

(Dated: March 1, 2023)

## I. EXPERIMENTAL SETUP

A detailed scheme of the setup is shown in Fig. S1. The experiment has been performed in a custom-built wet dilution cryostat. A Zurich Instruments HDAWG 750 MHz arbitrary waveform generator provides modulation pulses to radio frequency (RF) sources (R&S SGS100A) and for synchronizing the Field Programmable Gate Array (FPGA, model NI PXIe 7972). The RF sources are referenced to each other in a daisy chain configuration at a frequency of 1000 MHz starting with the RF source connected to In2. This source, the AWG and the FPGA are synchronized at a frequency of 10 MHz by means of a rubidium frequency standard (Stanford Research Systems FS725). The different input lines (In1, In2, P1, P2) are sequentially attenuated at various temperature stages. The coldest attenuator of In1 (In2) is thermally coupled to a 100-Ω heater and a $RuO_2$ temperature sensor. At the same time, the attenuator is only weakly coupled to the mixing chamber plate of the dilution refrigerator. This allows for a precise PID temperature control of the coldest attenuators, while all other components can remain stable at a base temperature of $T = 35\,\mathrm{mK}$. The photon numbers in the reconstructed states are calibrated using Planck spectroscopy [2]. For that, we vary the temperature of a heatable 30-dB attenuator between 50 mK and 430 mK. The heatable attenuator serves as a self-calibrated, black-body photon source. This way, we can link the detected voltage at the FPGA to the set temperature or, equivalently, to a thermal photon number in a microwave signal emitted from the heatable attenuator [2]. The sample stage is surrounded by a Cryoperm shield to protect it from magnetic stray field. In addition, JPA2 is enclosed in a superconducting Al-shield in order to avoid cross-talk between magnetic coils mounted onto the two JPAs. Due to the low signal level, both signals at the output of the cryogenic sample stage need amplification in multiple stages starting with a cryogenic high-electron-mobility transistor (HEMT) amplifier and subsequent additional room-temperature amplifiers. Frequency-resolved measurements are performed using a vector network analyzer (VNA, not shown).

The tomography of quantum microwave states is performed using a heterodyne receiver setup and data processing similar to previous experiments in Refs. [3–6]. Output signals at the operating frequency of 5.48 GHz are down-converted to an intermediate frequency of 11 MHz using image rejection mixers in combination with a local oscillator (LO) driven at 5.491 GHz. After the down-conversion, the signal power is adjustable by step attenuators in order to balance the two receiver lines. This attenuation also prevents compression effects in the subsequent amplification. After amplification and filtering, the down-converted signals are digitized by a transceiver adapter module (NI 5782-02) and processed in the FPGA. After digital down-conversion, the dc signals are further filtered by using a digital finite-impulse-response (FIR) filter with a full bandwidth of 400 kHz. From the filtered and digitized data we compute the quadrature moments $\langle I_1^n Q_1^m I_2^k Q_2^l \rangle$ with $n, m, k, l \leq 4$. We assume that all reconstructed states are Gaussian, i.e., that they are represented by a Gaussian characteristic function in the signal quadrature phase space and can be entirely described by first- and second-order moments of the quadrature operators [7]. This assumption can be verified by calculating third- and fourth-order cumulants which are expected to vanish for Gaussian states [8]. If these cumulants are much smaller than the first- and second-order cumulants, we conclude that the Gaussian-state

* fabian.kronowetter@wmi.badw.de

† kirill.fedorov@wmi.badw.de

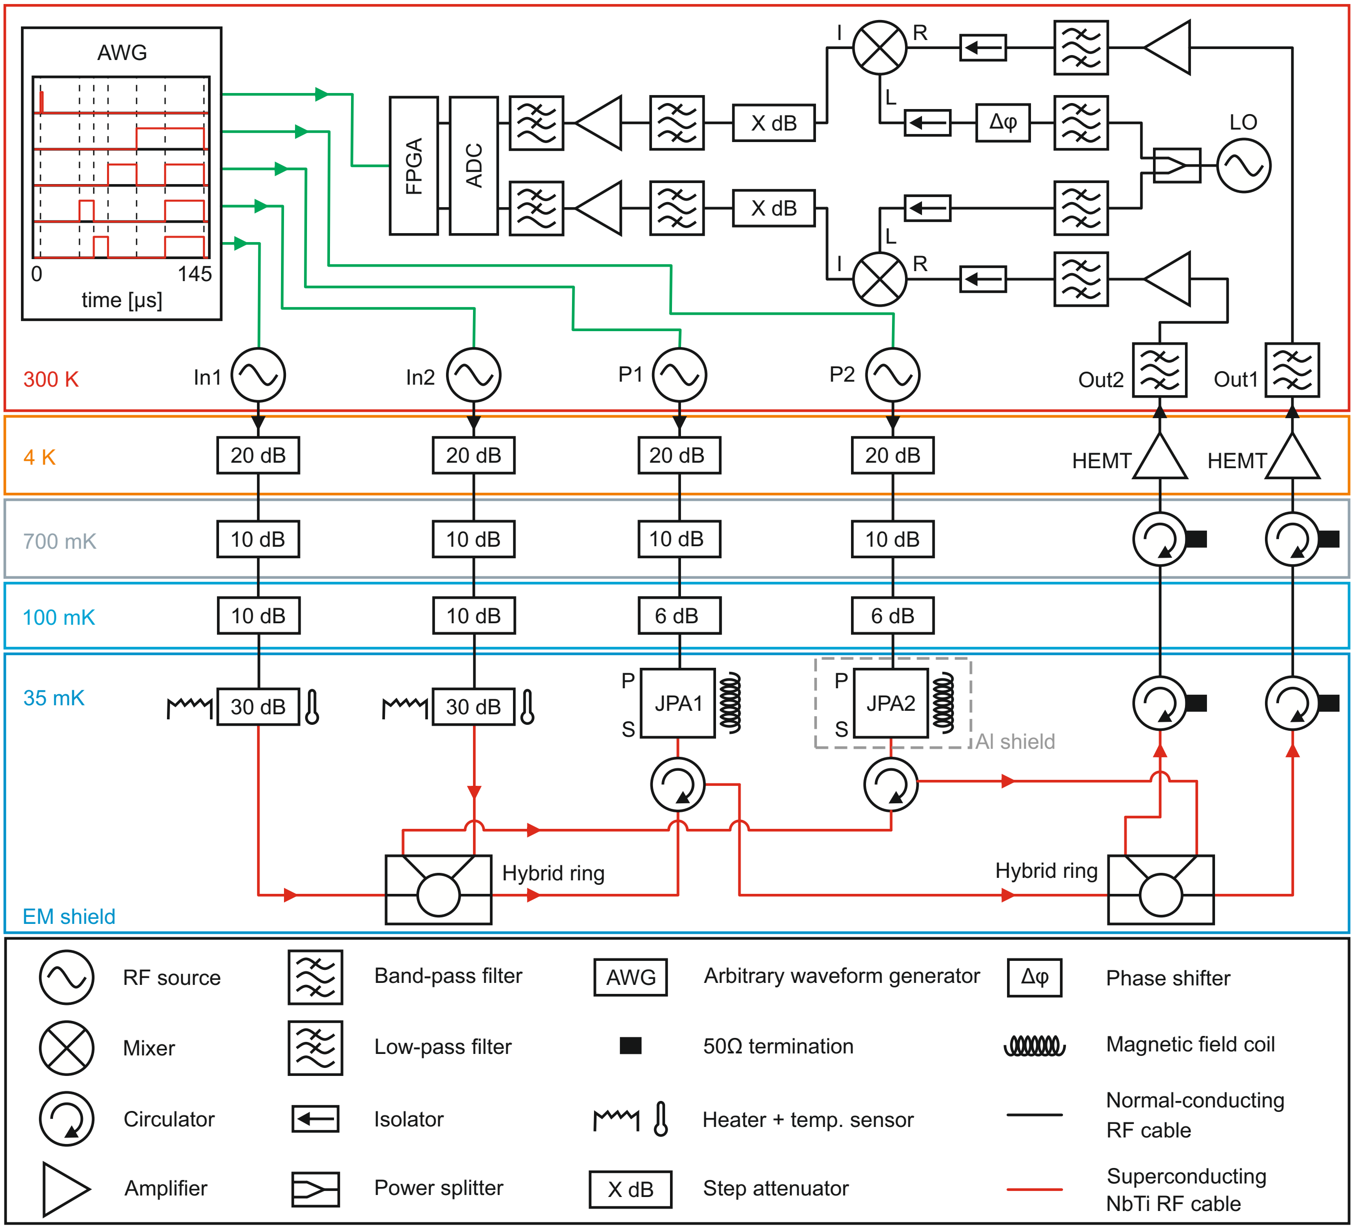


Figure S1. Schematic of the measurement setup. The output signals are amplified and filtered in subsequent steps, down-converted and digitized. An arbitrary waveform generator (AWG) creates a pulse sequence for the indivdual RF sources and the FPGA, which is required for the reference-state reconstruction [1].

approximation is appropriate. The JPA squeezing angles are set via a phase-locked loop, where in each measurement cycle the actual squeezing orientation $\gamma_i^{\mathrm{exp}}$ $(i = 1, 2)$ is extracted from the quadrature moments of the signals emitted from the respective JPA. Next, the phase of the corresponding JPA pump signal is adjusted by $2\Delta\gamma_i$, where $\Delta\gamma_i$ is the difference between the actual angle $\gamma_i^{\mathrm{exp}}$ and the target angle $\gamma_i^{\mathrm{target}}$. The respective phases of the coherent input tones are stabilized in a similar way by computing $\Delta\theta_i = \theta_i^{\mathrm{exp}} - \theta_i^{\mathrm{target}}$ and corrected by $\Delta\theta_i$. For independent adjustment of each RF source, the AWG produces a pulse sequence which drives each source twice per sequence: first for individual phase adjustment and the second time for data acquisition. A general scheme of the AWG pulse sequence is depicted in the inset in Fig. S1.

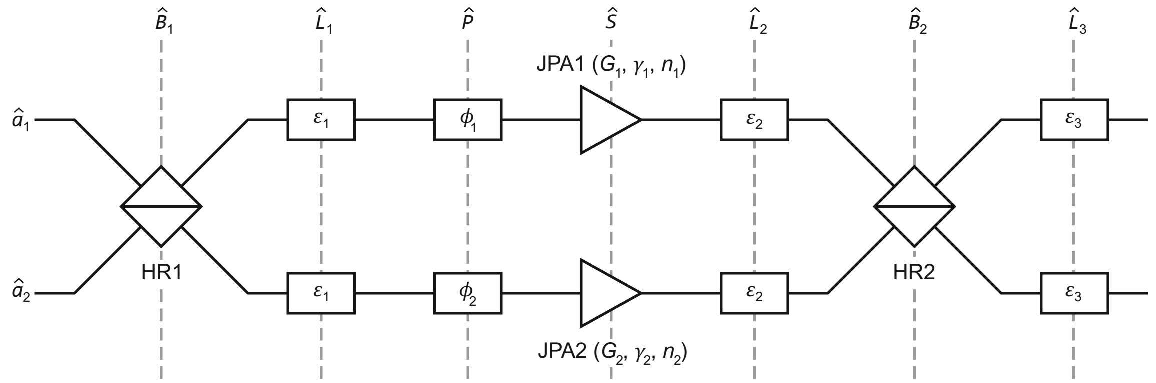


Figure S2. Scheme of the theoretical model of the interferometer circuit. The incoming modes $\hat{a}_1$ and $\hat{a}_2$ sequentially undergo various transformations, as indicated by the vertical dashed lines. The final states are reconstructed after the operation $\hat{L}_3$.

## II. THEORETICAL MODEL

The nonlinear interferometer is modeled in a step-wise approach as a sequence of different operations, as depicted in Fig. S2. Since the thermal population of our states with a frequency of $\omega/2\pi = 5.48\,\mathrm{GHz}$ at an effective temperature of $T \simeq 50\,\mathrm{mK}$ is small $[n_{\mathrm{th}} = 1/(\exp(\hbar\omega/k_{\mathrm{B}}T) - 1) \approx 5 \cdot 10^{-3} \ll 1]$, we assume vacuum fluctuations as the variance of both signal inputs. The initial coherent state $\hat{a}_i$ $(i = 1, 2)$ with complex displacement amplitude $\alpha_i$ is modeled by applying the displacement operator $\hat{D}(\alpha_i)$ to vacuum $\hat{v}_i$

$$\hat{a}_i = \hat{v}_i + \alpha_i. \tag{S1}$$

First, the signals of the two input lines are superimposed at a 180° hybrid ring, which we model as

$$\hat{B}_i^\dagger \begin{pmatrix} \hat{a}_1 \\ \hat{a}_2 \end{pmatrix} \hat{B}_i = \frac{1}{\sqrt{2}} \begin{pmatrix} -1 & 1 \\ 1 & 1 \end{pmatrix} \begin{pmatrix} \hat{a}_1 \\ \hat{a}_2 \end{pmatrix}, \tag{S2}$$

with $i \in \{1, 2\}$. The losses due to insertion, connectors and cable losses are modeled with a non-unitary operation according to

$$\hat{L}_j^\dagger \begin{pmatrix} \hat{a}_1 \\ \hat{a}_2 \end{pmatrix} \hat{L}_j = \begin{pmatrix} \sqrt{1-\varepsilon_j}\,\hat{a}_1 + \sqrt{\varepsilon_j}\,\hat{v}_1 \\ \sqrt{1-\varepsilon_j}\,\hat{a}_2 + \sqrt{\varepsilon_j}\,\hat{v}_2 \end{pmatrix}, \tag{S3}$$

with $j \in \{1, 2, 3\}$. The phase $\phi_i$ which is acquired by the signals in each interferometer arm is modeled as

$$\hat{P}^\dagger \begin{pmatrix} \hat{a}_1 \\ \hat{a}_2 \end{pmatrix} \hat{P} = \begin{pmatrix} e^{i\phi_1} & 0 \\ 0 & e^{i\phi_2} \end{pmatrix} \begin{pmatrix} \hat{a}_1 \\ \hat{a}_2 \end{pmatrix}. \tag{S4}$$

Next, the two JPAs perform a phase-sensitive amplification which we model by a squeezing operator according to

$$\hat{S}^\dagger \begin{pmatrix} \hat{a}_1 \\ \hat{a}_2 \end{pmatrix} \hat{S} = \\ = \begin{pmatrix} (\hat{a}_1 + \zeta_1)\cosh r_1 - \left(\hat{a}_1^\dagger + \zeta_1^*\right) e^{-2i\gamma_1} \sinh r_1 \\ (\hat{a}_2 + \zeta_2)\cosh r_2 - \left(\hat{a}_2^\dagger + \zeta_2^*\right) e^{-2i\gamma_2} \sinh r_2 \end{pmatrix}, \tag{S5}$$

where the JPA gain $G_i$ is related to the squeezing parameter $r_i$ via $G_i = e^{2r_i}$. The respective squeezing angle is denoted by $\gamma_i$. The noise added by the two JPAs is taken into account by introducing a random classical variable $\zeta_i$ which fulfills $\langle \zeta_i \zeta_i^* \rangle = n_i(G_i)$ and $\langle \mathrm{Re}\left(\zeta^2\right) \rangle = \langle \mathrm{Im}\left(\zeta^2\right) \rangle = n_i(G_i)/2$. Note that the noise is depending on the respective gain [9]. For reliable analysis of $G_i$ and $n_i$, we reconstruct the corresponding quantum states at the output of the second HR in a frame of the AWG pulsing scheme, when only JPA1 (JPA2) is driven, as depicted in Fig. S1. The full transformation of the circuit is given by the combined operator

$$\hat{F} = \hat{L}_3 \hat{B}_2 \hat{L}_2 \hat{S} \hat{P} \hat{L}_1 \hat{B}_1. \tag{S6}$$

Consequently, the final state $|\Psi\rangle$ can be expressed as [10]

$$|\Psi\rangle = \hat{F}|\alpha_1;\alpha_2\rangle. \tag{S7}$$

The signal moments of the circuit outputs $\hat{b}_i$ are given by

$$\begin{pmatrix} \langle(\hat{b}^\dagger)^n\hat{b}^m\rangle_1 \\ \langle(\hat{b}^\dagger)^n\hat{b}^m\rangle_2 \end{pmatrix} = \langle\Psi| \begin{pmatrix} \langle(\hat{a}^\dagger)^n\hat{a}^m\rangle_1 \\ \langle(\hat{a}^\dagger)^n\hat{a}^m\rangle_2 \end{pmatrix} |\Psi\rangle. \tag{S8}$$

Since we are exclusively considering Gaussian states, we restrict ourselves to signal moments up to the second order [11]. They are obtained by applying the operator of Eq. (S6) to the initial signal moments with $m+n \leq 2$. With the complementary quadrature operators given by

$$\hat{q} = \frac{\hat{a}+\hat{a}^\dagger}{2}, \tag{S9}$$

$$\hat{p} = \frac{\hat{a}-\hat{a}^\dagger}{2i}, \tag{S10}$$

we define the vector $\hat{\mathbf{r}} = (\hat{q}_1, \hat{p}_1, \hat{q}_2, \hat{p}_2)$ containing the quadrature pairs of two modes, in our case. Gaussian states are fully described by the displacement vector $\hat{d}_i = \langle\hat{r}_i\rangle$ and the covariance matrix $V_{ij} = \langle\hat{r}_i\hat{r}_j + \hat{r}_j\hat{r}_i\rangle/2 - \langle\hat{r}_i\rangle\langle\hat{r}_j\rangle$, for $i,j \in \{1,2,3,4\}$.

All quantities discussed in the main text are either evaluated directly with the signal moments, the associated first and second statistical moments, or by using the second-order correlation function [12] and Gaussian interferometric power [7]. Here, we combine our model with the approach from Ref. [12] to express second-order correlation functions for arbitrary Gaussian states based on their respective covariance matrix and displacement vector. The second-order auto-correlation functions $g_1^{(2)}(0)$ and $g_2^{(2)}(0)$, as well as the second-order cross-correlation function $g_\mathrm{C}^{(2)}(0)$ are given by

$$\begin{aligned} g_1^{(2)}(0) = 2 \Bigg[ 2 \Bigg( 2\,(V_{11}+V_{22})^2 + 4\,(V_{11}+V_{22}) \left(\frac{|d_1+i\,d_2|}{\sqrt{2}}\right)^2 + \left( |\,(V_{11}-V_{22}-2i\,V_{12}) + \left(\frac{|d_1+i\,d_2|}{\sqrt{2}}\right)^2 | \right)^2 \Bigg) \\ -4 \left( V_{11}+V_{22} + \left(\frac{|d_1+i\,d_2|}{\sqrt{2}}\right)^2 \right) + 1 \Bigg] \Big/ \left[ \left( 2 \left( V_{11}+V_{22} + \left(\frac{|d_1+i\,d_2|}{\sqrt{2}}\right)^2 \right) - 1 \right)^2 \right], \end{aligned} \tag{S11}$$

$$\begin{aligned} g_2^{(2)}(0) = 2 \Bigg[ 2 \Bigg( 2\,(V_{33}+V_{44})^2 + 4\,(V_{33}+V_{44}) \left(\frac{|d_3+i\,d_4|}{\sqrt{2}}\right)^2 + \left( |\,(V_{33}-V_{44}-2i\,V_{34}) + \left(\frac{|d_3+i\,d_4|}{\sqrt{2}}\right)^2 | \right)^2 \Bigg) \\ -4 \left( V_{33}+V_{44} + \left(\frac{|d_3+i\,d_4|}{\sqrt{2}}\right)^2 \right) + 1 \Bigg] \Big/ \left[ \left( 2 \left( V_{33}+V_{44} + \left(\frac{|d_3+i\,d_4|}{\sqrt{2}}\right)^2 \right) - 1 \right)^2 \right], \end{aligned} \tag{S12}$$

$$g_{\mathrm{C}}^{(2)}(0) = \frac{2\,(A+B)^2 - 3\,B - 3\,a - 3\,b + \left|A - B - 2i\,C + \frac{(x_2+i\,y_2)^2}{2}\right|^2 + \frac{|x_1+i\,y_1|^2\,|x_2+i\,y_2|^2}{2}}{\left(\frac{|x_1+i\,y_1|^2}{2} + \frac{|x_2+i\,y_2|^2}{2} + A + B + a + b - 1\right)^2}$$
$$+ \frac{-3\,A + 2\,(a+b)\,(A+B) - \frac{3\,|x_1+i\,y_1|^2}{2} - \frac{3\,|x_2+i\,y_2|^2}{2} + \frac{|x_2+i\,y_2|^2\,(4\,A+4\,B)}{2} + \left|a - b - 2i\,c + \frac{(x_1+i\,y_1)^2}{2}\right|^2}{\left(\frac{|x_1+i\,y_1|^2}{2} + \frac{|x_2+i\,y_2|^2}{2} + A + B + a + b - 1\right)^2}$$
$$+ \frac{2\,|e + h + i\,f - i\,g|^2 + 2\,(a+b)^2 + \frac{|x_1+i\,y_1|^2\,(4\,a+4\,b)}{2} + |x_1 + i\,y_1|^2\,(A+B) + 2\,|h - e + i\,f + i\,g|^2}{\left(\frac{|x_1+i\,y_1|^2}{2} + \frac{|x_2+i\,y_2|^2}{2} + A + B + a + b - 1\right)^2}$$
$$+ \frac{|x_2 + i\,y_2|^2\,(a+b) + (x_1 - i\,y_1)\,(x_2 + i\,y_2)\,(e + h - i\,f + i\,g)}{\left(\frac{|x_1+i\,y_1|^2}{2} + \frac{|x_2+i\,y_2|^2}{2} + A + B + a + b - 1\right)^2}$$
$$+ \frac{(x_1 + i\,y_1)\,(x_2 - i\,y_2)\,(e + h + i\,f - i\,g) - (x_1 - i\,y_1)\,(x_2 - i\,y_2)\,(h - e + i\,f + i\,g)}{\left(\frac{|x_1+i\,y_1|^2}{2} + \frac{|x_2+i\,y_2|^2}{2} + A + B + a + b - 1\right)^2}$$
$$+ \frac{(x_1 + i\,y_1)\,(x_2 + i\,y_2)\,(e - h + i\,f + i\,g) + \frac{3}{2}}{\left(\frac{|x_1+i\,y_1|^2}{2} + \frac{|x_2+i\,y_2|^2}{2} + A + B + a + b - 1\right)^2}, \tag{S13}$$

where

$$a = V_{11},\ b = V_{22},\ c = V_{12},\ e = V_{13},\ f = V_{14},\ g = V_{23},\ h = V_{24},\ A = V_{33},\ B = V_{44},\ C = V_{34}, \tag{S14}$$

and

$$x_1 = d_1,\ y_1 = d_2,\ x_2 = d_3,\ y_2 = d_4. \tag{S15}$$

The Gaussian interferometric power can be expressed as [7]

$$\mathcal{P} = \frac{\left(X + \sqrt{X^2 + YZ}\right)}{2Y}, \tag{S16}$$

where

$$X = (D+F)\cdot(1+E+F-G) - G^2, \tag{S17}$$
$$Y = (G-1)\cdot(1+D+E+2F+G), \tag{S18}$$
$$Z = (D+G)\cdot(D\cdot E - G) + F(2D+F)\cdot(1+E), \tag{S19}$$

and

$$D = 4(V_{11}V_{22} - V_{12}V_{21}), \tag{S20}$$
$$E = 4(V_{33}V_{44} - V_{34}V_{43}), \tag{S21}$$
$$F = 4(V_{13}V_{24} - V_{14}V_{23}), \tag{S22}$$
$$G = \det(4\mathbf{V}). \tag{S23}$$

In the main text, we used the theoretical (reconstructed) photon number of the local mode at Out1 of our circuit to compute $\mathcal{P}_{\mathrm{SQL}} = N = \left(2(\sigma_q^2 + \sigma_p^2) - 1\right)/2$ and $\mathcal{P}_{\mathrm{HL}}$.

The parameters used in the theoretical model are summarized in Tables S1 and S2. The parameters $\varepsilon_1$, $\varepsilon_2$ and $\varepsilon_3$ are estimated from the data sheets of the respective passive microwave components. The displacement amplitudes $|\alpha_1|$ and $|\alpha_2|$ are adjusted via the photon number calibration factor in combination with an individual two-pulsed power sweep of the two RF sources connected to In1 and In2. The displacement angles $\theta_1$ and $\theta_2$ in Table S1 (Table S2) are reconstructed and adjusted in real time using $6.248 \cdot 10^8$ ($9.372 \cdot 10^8$) raw data points. The squeezing angles $\gamma_1$ and $\gamma_2$ in Table S1 (Table S2) are processed similarly using $1.2496 \cdot 10^9$ ($1.8744 \cdot 10^9$) raw data points. The reconstructed JPA squeezing factors, $r_1$ and $r_2$, are obtained in post-processing, where the averaged demodulated data is taken into account for 46 independent measurements of $1.2496 \cdot 10^9$ ($1.8744 \cdot 10^9$) raw data points, respectively. The theory model relies on $\phi_i$ as free parameter, representing the phase acquired by signals in paths 1 and 2 of the interferometer, respectively.

| $\|\alpha_1\|^2$ | $\theta_1$ | $\|\alpha_2\|^2$ | $\theta_2$ | $\varepsilon_1$ (dB) | $\phi_1$ | $\phi_2$ | $r_1$ | $\gamma_1$ | $n_1$ | $r_2$ | $\gamma_2$ | $n_2$ | $\varepsilon_2$ (dB) | $\varepsilon_3$ (dB) |
|---|---|---|---|---|---|---|---|---|---|---|---|---|---|---|
| 0.723 | $0.639\pi$ | 0.670 | 0 to $2\pi$ | 0.63 | $1.31\pi$ | $1.36\pi$ | 1.01(4) | 0 to $2\pi$ | 0.034(5) | 0.723(2) | 0 | 0.441(9) | 0.31 | 0.3 |

Table S1. Model parameters used for the simulated results of Figs. 3 and 4 in the main text. Each point in Figs. 3 and 4 in the main text is obtained using $1.4 \cdot 10^9$ raw data points. The loss values $\varepsilon_j$ are estimated based on the respective data sheet values. The complex displacement amplitudes $\alpha_i = |\alpha_i| \exp[i(\pi/2 - \theta_i)]$ and the respective JPA parameters $(r_i,\, n_i,\, \gamma_i)$ are reconstructed.

| $\|\alpha_1\|^2$ | $\theta_1$ | $\|\alpha_2\|^2$ | $\theta_2$ | $\varepsilon_1$ (dB) | $\phi_1$ | $\phi_2$ | $r_1$ | $\gamma_1$ | $n_1$ | $r_2$ | $\gamma_2$ | $n_2$ | $\varepsilon_2$ (dB) | $\varepsilon_3$ (dB) |
|---|---|---|---|---|---|---|---|---|---|---|---|---|---|---|
| 0.177 to 10.76 | $0.806\pi$ | 0.177 to 10.76 | $0.806\pi$ | 0.63 | $1.03\pi$ | $1.36\pi$ | 0.508(5) | $\pi/2$ | 0.0004(6) | 0.422(5) | $\pi$ | 0.124(4) | 0.31 | 0.3 |

Table S2. Model parameters used for the simulated results of Fig. 5 in the main text. Each point in Fig. 5 in the main text is obtained using $2.1 \cdot 10^9$ raw data points per independent measurement. The shown values are derived in the same way as in Table S1 and averaged for 16 independent measurements.

## III. CIRCUIT CALIBRATION

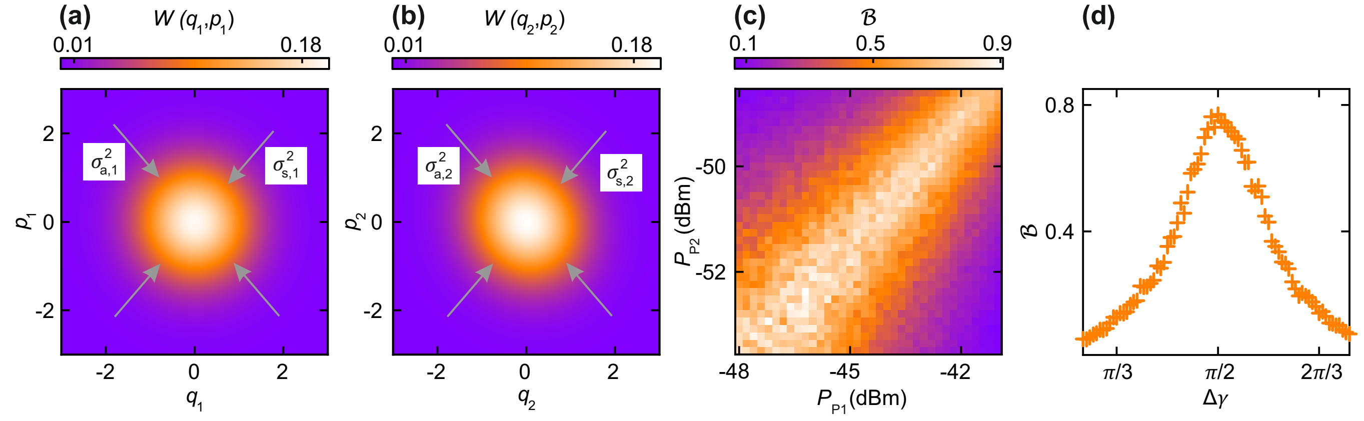


Figure S3. Interferometer calibration. The squashed variances $\sigma^2_{\mathrm{s},i}$ and amplified variances $\sigma^2_{\mathrm{a},i}$ $(i = 1, 2)$ of the reconstructed Wigner functions $W(q_i, p_i)$ of the output fields in (a) Out1 and (b) Out2 are used to define a balancing parameter $\mathcal{B}$, which enables optimization of (c) JPA pump powers $P_{\mathrm{P1}}$ and $P_{\mathrm{P2}}$ (at the JPA ports) and (d) a relative JPA amplification orientation $\Delta\gamma = |\gamma_1 - \gamma_2|$.

Figure S3 illustrates the concept behind the balancing parameter $\mathcal{B} = \left(\sigma^2_{\mathrm{s},1}/\sigma^2_{\mathrm{a},1}\right)\cdot\left(\sigma^2_{\mathrm{s},2}/\sigma^2_{\mathrm{a},2}\right)$. Figure S3(a) shows the reconstructed Wigner function of the local output Out1 of the interferometer during calibration. We analyze remaining variance asymmetries between two orthogonal quadratures $\sigma^2_{\mathrm{a},1}$ and $\sigma^2_{\mathrm{s},1}$ and try to minimize them. Similarly, as shown in Fig. S3(b), we optimize $\sigma^2_{\mathrm{a},2}$ versus $\sigma^2_{\mathrm{s},2}$. For a fixed $\Delta\gamma_{\mathrm{JPA}} = \pi/2$, we investigate $\mathcal{B}$ as a function of the level of the pump tones, $P_{\mathrm{P1}}$ and $P_{\mathrm{P2}}$, entering the respective JPA pump port [Fig. S3(c)]. As can be seen in Fig. S3(d), the balancing is best for amplification along orthogonal orientations in phase space, i.e., $\Delta\gamma_{\mathrm{JPA}} = |\gamma_2 - \gamma_1| = \pi/2$, as expected from theory [11].


[1] E. P. Menzel, R. Di Candia, F. Deppe, P. Eder, L. Zhong, M. Ihmig, M. Haeberlein, A. Baust, E. Hoffmann, D. Ballester, K. Inomata, T. Yamamoto, Y. Nakamura, E. Solano, A. Marx, and R. Gross, Path entanglement of continuous-variable quantum microwaves, Physical Review Letters **109**, 250502 (2012).

[2] M. Mariantoni, E. P. Menzel, F. Deppe, M. A. Araque Caballero, A. Baust, T. Niemczyk, E. Hoffmann, E. Solano, A. Marx, and R. Gross, Planck spectroscopy and quantum noise of microwave beam splitters, Physical Review Letters **105**, 133601 (2010).

[3] M. Renger, S. Pogorzalek, F. Fesquet, K. Honasoge, F. Kronowetter, Q. Chen, Y. Nojiri, K. Inomata, Y. Nakamura, A. Marx, F. Deppe, R. Gross, and K. G. Fedorov, Flow of quantum correlations in noisy two-mode squeezed microwave states, Physical Review A **106**, 052415 (2022).
[4] S. Pogorzalek, K. G. Fedorov, M. Xu, A. Parra-Rodriguez, M. Sanz, M. Fischer, E. Xie, K. Inomata, Y. Nakamura, E. Solano, A. Marx, F. Deppe, and R. Gross, Secure quantum remote state preparation of squeezed microwave states, Nature Communications **10**, 2604 (2019).
[5] K. G. Fedorov, S. Pogorzalek, U. Las Heras, M. Sanz, P. Yard, P. Eder, M. Fischer, J. Goetz, E. Xie, K. Inomata, Y. Nakamura, R. Di Candia, E. Solano, A. Marx, F. Deppe, and R. Gross, Finite-time quantum entanglement in propagating squeezed microwaves, Scientific Reports **8**, 6416 (2018).
[6] K. G. Fedorov, M. Renger, S. Pogorzalek, R. Di Candia, Q. Chen, Y. Nojiri, K. Inomata, Y. Nakamura, M. Partanen, A. Marx, R. Gross, and F. Deppe, Experimental quantum teleportation of propagating microwaves, Science Advances **7**, eabk0891 (2021).
[7] G. Adesso, Gaussian interferometric power, Physical Review A **90**, 022321 (2014).
[8] S.-H. Xiang, W. Wen, Y.-J. Zhao, and K.-H. Song, Evaluation of the non-Gaussianity of two-mode entangled states over a bosonic memory channel via cumulant theory and quadrature detection, Physical Review A **97**, 042303 (2018).
[9] M. Renger, S. Pogorzalek, Q. Chen, Y. Nojiri, K. Inomata, Y. Nakamura, M. Partanen, A. Marx, R. Gross, F. Deppe, and K. G. Fedorov, Beyond the standard quantum limit for parametric amplification of broadband signals, npj Quantum Information **7**, 160 (2021).
[10] Note that this is only a symbolic notation for better clarity. For a full description, the environment enters via two additional modes. Since we do not care further about the environment, we drop these modes.
[11] S. L. Braunstein and P. van Loock, Quantum information with continuous variables, Reviews of Modern Physics **77**, 513 (2005).
[12] S. Olivares, S. Cialdi, and M. G. Paris, Homodyning the $g^{(2)}(0)$ of Gaussian states, Optics Communications **426**, 547 (2018).
